# Supplementary material for: NegFaceDiff: The Power of Negative Context in Identity-Conditioned Diffusion for Synthetic Face Generation
Source: arXiv:2508.09661 source file (2025-08-13)
Supplement: Supplementary file 1 [file supplementary.pdf]

# NegFaceDiff: The Power of Negative Context in Identity-Conditioned Diffusion for Synthetic Face Generation

## Supplementary Material

### 1. Ablation Study on $w$

#### 1.1. Experimental Setup

The introduction of a negative context in the diffusion model’s sampling process requires defining a value for  $w$ , the hyperparameter that weights the negative context’s influence. The value of  $w$  was selected by fixing one of the proposed NegFaceDiff negative context selection strategies, Far-Neg, and using it to generate datasets associated with distinct  $w$  values ( $w = \{0.25, 0.50, 1.00\}$ ). These datasets were then used to train FR systems, in order to assess which  $w$  value results in a dataset better prepared for FR training. The sampling process followed DDIM (200 steps) and FR was performed with no data augmentation and following the same setup as the remaining experiments on the paper.

#### 1.2. Results

Table 1 presents the results of the ablation study on the value of  $w$ . The value assigned to  $w$  during the sampling process has a significant impact in the performance achieved by FR models trained on the generated data, as shown by the significant performance gap of 6.43% percentage points between the worst ( $w = 1$ ) and best ( $w = 0.5$ ) performing values. Given these results, we fixed  $w = 0.5$  for all the remaining experiments. It should also be noted that NegFaceDiff with  $w = 0.5$  reached higher FR performance than the baseline method, IDiff-Face [1], for which no negative condition is used.

| Method         | $w$  | Verification Benchmarks $\uparrow$ |              |              |              |              |              |
|----------------|------|------------------------------------|--------------|--------------|--------------|--------------|--------------|
|                |      | LFW                                | Cross-Age    |              | Cross-Pose   |              | Average      |
|                |      |                                    | AgeDB-30     | CA-FLW       | CFP-FP       | CP-LFW       |              |
| IDiff-Face [1] | 0    | 96.30                              | 78.15        | 86.23        | 81.51        | 77.57        | 83.95        |
| NegFaceDiff    | 0.25 | 96.63                              | 78.55        | 86.62        | <b>82.04</b> | 78.20        | 84.41        |
|                | 0.50 | <b>96.78</b>                       | <b>81.35</b> | <b>87.67</b> | 81.89        | <b>78.43</b> | <b>85.22</b> |
|                | 1.0  | 92.82                              | 73.98        | 80.22        | 74.81        | 72.10        | 78.79        |

Table 1. Verification accuracies (in %) on five FR benchmarks for models trained on 500k samples (10k identities with 50 images per identity) generated using Far-Neg with different weights for the negative context,  $w$ . IDiff-Face [1] results are presented as a baseline that does not include negative conditions in the generation process ( $w = 0$ ). The best accuracy is marked in **bold**.

## References

- [1] Fadi Boutros, Jonas Henry Grebe, Arjan Kuijper, and Naser Damer. Idiff-face: Synthetic-based face recognition through fuzzy identity-conditioned diffusion models. In *IEEE/CVF International Conference on Computer Vision, ICCV 2023, Paris, France, October 1-6, 2023*, pages 19593–19604. IEEE, 2023. [1](#)
